# Supplementary material for: Quantum Monte Carlo study of lattice polarons in the two-dimensional multi-orbital Su-Schrieffer-Heeger model
Source: arXiv:1901.07612 source file (2019-01-22)
Supplement: Supplementary file 1 [file supplementary.pdf]

# Quantum Monte Carlo study of lattice polarons in the two-dimensional multi-orbital Su-Schrieffer-Heeger model – Supplementary Materials

Shaozhi Li[1,2] and Steven Johnston[1,3,*]

[1]*Department of Physics and Astronomy, The University of Tennessee, Knoxville, Tennessee 37996, USA*

[2]*Department of Physics, University of Michigan, Ann Arbor, Michigan 48109, USA*

[3]*Joint Institute for Advanced Materials at The University of Tennessee, Knoxville, Tennessee 37996, USA*

(Dated: January 19, 2019)

* sjohn145@utk.edu

## S1. Treating the three-orbital Su-Schrieffer-Heeger model with determinant quantum Monte Carlo

This section provides the details of the determinant quantum Monte Carlo (DQMC) algorithm applied to the three-orbital Su-Schrieffer-Heeger (SSH) model and the standard measurements discussed in the main text. For additional discussion, the reader is directed to Refs. [S1] and [S2].

### S1.1. The DQMC Algorithm

DQMC computes the expectation value of an observable $\hat{O}$ in the grand canonical ensemble

$$\langle \hat{O} \rangle = \frac{\mathrm{Tr}\left[\hat{O}e^{-\beta H}\right]}{\mathrm{Tr}\left[e^{-\beta H}\right]}, \tag{S1}$$

where $Z = \mathrm{Tr}\left[e^{-\beta H}\right]$ is the partition function. We will use $Z$ as an example to illustrate the method since generalizations to the operator $\hat{O}$ are straightforward [S1].

The first step is to divide the imaginary time interval $[0, \beta]$ into $L$ discrete steps of length $\Delta\tau = \beta/L$ such that the partition function can be rewritten using the Trotter formula

$$Z = \mathrm{Tr}\left(e^{-\Delta\tau L H}\right) \approx \mathrm{Tr}\left(e^{-\Delta\tau H_{e-ph}}e^{-\Delta\tau K}\right)^L,$$

where $K$ contains the noninteracting terms of the Hamiltonian $K = H_0 + H_{\mathrm{lat}}$ and $H_{e-ph}$ contains the $e$-ph interaction. The Trotter approximation neglects terms of order $\mathcal{O}(\Delta\tau)^2$, which is controllable as $\Delta\tau \to 0$.

Next, the phonon operators are treated by inserting a complete set of position and momentum eigenstates at each time slice. One then integrates out the phonon momenta analytically such that the partition function depends only on a trace over the continuous lattice displacements $X_{\mathbf{r},x}$ and $X_{\mathbf{r},y}$ and terms that are bilinear in the Fermion operators. The trace over the Fermion degrees of freedom can then be evaluated analytically and expressed as a product of matrix determinants [S3]. The final result is

$$Z = \int dX_x \int dX_y e^{-S_{ph}\Delta\tau}\det\left[M_\uparrow\right]\det\left[M_\downarrow\right], \tag{S2}$$

where $\int dX_x$ and $\int dX_y$ are shorthand for multidimensional integrals over the displacements

$X_{\mathbf{r},x,l}$ and $X_{\mathbf{r},y,l}$ defined at each oxygen site and time slice $l$. The matrix $M_\sigma$ is defined as $M_\sigma = I + B_\sigma(L)B_\sigma(L-1)\cdots B_\sigma(1)$, where $I$ is an $N \times N$ identity matrix and the $B_\sigma(l)$ matrices are defined as $B_\sigma(l) = e^{-\Delta\tau H_{e-ph}}e^{-\Delta\tau H_0}$. (Each $B_\sigma(l)$ is independent of $\sigma$ in this case.) Note that $H_{e-ph}$ has off-diagonal terms in orbital space due to the nature of the SSH interaction, unlike the case of the Holstein model where it is a diagonal matrix. The lattice contribution to the action is defined as

$$S_{ph} = KX^2_{\mathbf{r},x,l} + KX^2_{\mathbf{r},y,l} + \frac{M}{2}\left(\frac{X_{\mathbf{r},x,l+1} - X_{\mathbf{r},x,l}}{\Delta\tau}\right)^2 + \frac{M}{2}\left(\frac{X_{\mathbf{r},y,l+1} - X_{\mathbf{r},y,l}}{\Delta\tau}\right)^2. \quad \text{(S3)}$$

The final step is to evaluate the displacement integrals using Metropolis sampling. In this work, we performed both single-site and block updates [S2], as described below.

Most observables can be expressed in terms of the single particle Green's function $G_\sigma(\tau)$. For an electron propagating through field configurations $\{X_{\mathbf{r},x,l}\}$ and $\{X_{\mathbf{r},y,l}\}$, the Green's function at time $\tau = l\Delta\tau$ is given by

$$[G_\sigma(l)]_{ij} = \langle \hat{T}_\tau c_{i,\sigma}(\tau)c^\dagger_{j,\sigma}(\tau)\rangle = [I + A_\sigma(l)]^{-1}_{ij}, \quad \text{(S4)}$$

where $A_\sigma(l) = B_\sigma(l)\cdots B_\sigma(1)B_\sigma(L)\cdots B_\sigma(l+1)$, $\hat{T}_\tau$ is the time ordering operator, and $i$, $j$ are combined orbital and site indicies. The determinant of $M_\sigma$ is related to the Green's function $M_\sigma = \det[G_\sigma(l)]^{-1}$ and is independent of $l$.

### S1.2. Efficient single-site updates

Equation (S4) shows that the Green's function $G^\sigma(l+1)$ can be obtained from $G_\sigma(l)$ using the identity

$$G_\sigma(l+1) = B_\sigma(l+1)G_\sigma(l)B^{-1}_\sigma(l+1). \quad \text{(S5)}$$

This observation forms the basis for an efficient single-site Sherman-Morris updating scheme [S1]. The DQMC algorithm starts by computing the Green's function on time slice $l = 0$ using Eq. (S4). A series of individual updates are then proposed by sweeping through the sites $(\mathbf{r}, \alpha = x, y)$ proposing updates $X_{\mathbf{r},\alpha,l} \rightarrow X'_{\mathbf{r},\alpha,l} = X_{\mathbf{r},\alpha,l} + \Delta X_{\mathbf{r},\alpha,l}$ while holding the other phonon fields $\{X_{\mathbf{r}'\neq\mathbf{r},\alpha'\neq\alpha,l}\}$ fixed. These updates are accepted with

probability $p = \min(1, R)$, where

$$R = e^{-\Delta\tau(S_{ph}[\{X'_{\mathbf{r},\alpha,l}\}]-S_{ph}[\{X_{\mathbf{r},\alpha,l}\}])} \frac{\det\left[M'_\uparrow\right]\det\left[M'_\downarrow\right]}{\det\left[M_\uparrow\right]\det\left[M_\downarrow\right]},$$

and $M'_\sigma$ and $M_\sigma$ correspond to matrices computed with the new and old phonon field configurations, respectively. Note that the product $\det[M_\uparrow]\det[M_\downarrow]$ is positive definite for the model considered here and *there is no Fermion sign problem.*

After updating a field $X_{\mathbf{r},\alpha,l}$, the corresponding $B_\sigma(l)$ matrix must also be updated as

$$B_\sigma(l) \to B'_\sigma(l) = e^{-\Delta\tau H'_{e-ph}} e^{-\Delta\tau H_0} = e^{-\Delta\tau(H_{e-ph}+V)} e^{-\Delta\tau H_0}, \tag{S6}$$

where $V$ contains the terms in $H_{e-ph}$ arising from the change in the phonon field. From the Hamiltonian, we can infer that $V$ is a symmetric matrix with only four non-zero elements and it can be written in the form

$$V = \begin{bmatrix} \ddots & \vdots & \vdots & \vdots & \vdots \\ \cdots & 0 & \alpha t^0_{sp}\Delta X_{\mathbf{r},l} & 0 & \cdots \\ \cdots & \alpha t^0_{sp}\Delta X_{\mathbf{r},l} & 0 & \alpha t^0_{sp}\Delta X_{\mathbf{r},l} & \cdots \\ \cdots & 0 & \alpha t^0_{sp}\Delta X_{\mathbf{r},l} & 0 & \cdots \\ \vdots & \vdots & \vdots & \vdots & \ddots \end{bmatrix}. \tag{S7}$$

To efficiently calculate the new $B'_\sigma(l)$ matrix, we make the approximation

$$B'_\sigma(l) \approx e^{-\Delta\tau V} B_\sigma(l), \tag{S8}$$

which introduces an error on the order of the Trotter error and is valid when $\Delta\tau$ is small. The matrix $e^{-\Delta\tau V}$ is then evaluated via $e^{-\Delta\tau V} = Pe^{-\Delta\tau D}P^T$, where $P$ is the orthogonal transformation that diagonalizes $V$, and $D$ is a diagonal matrix with only two non-zero elements $[D]_{11} = -\sqrt{2}\alpha t^0_{sp}\Delta X_{\mathbf{r},l}$ and $[D]_{NN} = \sqrt{2}\alpha t^0_{sp}\Delta X_{\mathbf{r},l}$. The $B'_\sigma(l)$ matrix can then be written as

$$B'_\sigma(l) = Pe^{-\Delta\tau D}P^T B_\sigma(l) = P(I+\Delta)P^T B_\sigma(l), \tag{S9}$$

where $[\Delta]_{ij} = 0$ except $[\Delta]_{11} = e^{\sqrt{2}\alpha t^0_{sp}\Delta X_{\mathbf{r},l}} - 1$ and $[\Delta]_{NN} = e^{-\sqrt{2}\alpha t^0_{sp}\Delta X_{\mathbf{r},l}} - 1$.

Using these approximations, the Green's function can be efficiently updated after accepting a change in the phonon field using

$$G'_\sigma(l) = [I + A'_\sigma(l)]^{-1} = \left[I + P(I+\Delta)P^T A_\sigma(l)\right]^{-1} = G^\sigma(l)\left[P^T + \Delta Q\right]^{-1} P^T, \qquad \text{(S10)}$$

where $Q = P^T[I - G_\sigma(l)]$. Due to the sparsity of matrix $\Delta$, $\Delta Q$ has only two non-zero rows

$$\begin{aligned}
\Delta Q &= \begin{bmatrix} \Delta_{1,1}Q_{1,1} & \Delta_{1,1}Q_{1,2} & \cdots & \Delta_{1,1}Q_{1,N} \\ 0 & 0 & \cdots & 0 \\ \vdots & \vdots & \vdots & \vdots \\ 0 & 0 & \cdots & 0 \\ \Delta_{N,N}Q_{N,1} & \Delta_{N,N}Q_{N,2} & \cdots & \Delta_{N,N}Q_{N,N} \end{bmatrix} \\
&= \begin{bmatrix} \Delta_{1,1} & 0 \\ \vdots & \vdots \\ 0 & \Delta_{N,N} \end{bmatrix} \times \begin{bmatrix} Q_{1,1} & Q_{1,2} & \cdots & Q_{1,N} \\ Q_{N,1} & Q_{N,2} & \cdots & Q_{N,N} \end{bmatrix} \\
&= uw,
\end{aligned} \qquad \text{(S11)}$$

where $u$ and $w$ are $N \times 2$ and $2 \times N$ matrices, respectively. Using the Woodbury matrix identity and Matrix determinant lemma, the updated Green's function is given by

$$G'_\sigma(l) = G_\sigma(l)\left[I - Pu(I_2 + vPw)^{-1}v\right], \qquad \text{(S12)}$$

and the acceptance ratio is given by

$$R_\sigma = \det\left[I_2 + wPu\right], \qquad \text{(S13)}$$

where $I_2$ is a $2 \times 2$ identity matrix. Evaluating these expressions involves $\mathcal{O}(N^2)$ operations, as opposed to computing the updated Green's function from scratch using Eq. (S4), which has a computational cost of $\mathcal{O}(N^3)$. Once updates have been performed for the fields on a given time slice $l$, $G_\sigma(l)$ is advanced to $G_\sigma(l+1)$ using Eq. (S5) and the process repeated.

This update scheme is efficient but it relies on the approximation $B'_\sigma(l) \approx e^{-\Delta\tau}B_\sigma(l)$. Section S1 S1.4 benchmarks this approach by comparing results obtained using our fast update method against results obtained by explicitly calculating $G'_\sigma(l)$. We find that the approximate fast update reproduces the exact solution with comparable error bars for $\Delta\tau$

values that are typical of most DQMC calculations.

### S1.3. Block updates

To reduce the autocorrelation time, we also periodically perform block updates of the phonon fields, where the lattice displacements for a given site are simultaneously updated on all imaginary time slices $l$. In other words, for a given $(\mathbf{r}, \alpha)$, the fields are updated as $X_{\mathbf{r},\alpha,l} \rightarrow X_{\mathbf{r},\alpha,l} + \Delta X_{\mathbf{r},\alpha}$ for all $\tau_l \in [0, \beta]$. This type of update efficiently moves phonon configurations out of false minima at low temperatures. There is, however, no fast method for updating Green's function following a block update; it must be calculated using Eq. (S4). As such, the inclusion of block updates slows down the simulations considerably. To strike a balance between the computational time and efficient sampling, we perform between two to four block updates at randomly selected sites for every full spacetime sweep of single-site updates.

### S1.4. Reliability of the fast updates

To assess the reliability of the approximation underlying Eq. (S8), we performed two DQMC calculations. In the first calculation, the updated Green's function following each single-site update and the acceptance ratio is computed exactly via Eqs. (S4) and (S6), respectively. In the second calculation, the fast update procedure is used following the single-site updates. Both calculations were carried out on a $2 \times 2$ cluster with a hole density $\langle \hat{n} \rangle = 1$. We further set $\beta = 6/t_{sp}$, $\Delta\tau = 1/10t_{ps}$, while the other parameters are the same as in the main text. Figure S1 shows that the Green's functions for both calculations are the same, indicating $\Delta\tau$ is small enough to reproduce the exact solution with comparable error bars.

## S2. Measurements

The dc conductivity is approximated using $\sigma_{\text{dc}} = \frac{\beta^2}{\pi}\Lambda_{xx}(\mathbf{q} = 0, \tau = \beta/2)$ [S4], where $\Lambda_{xx}(\mathbf{q}, \tau) = \sum_{\mathbf{r}} \langle \hat{j}_x(\mathbf{r}, \tau)\hat{j}_x(0, 0)\rangle e^{\mathrm{i}\mathbf{q}\cdot\mathbf{r}}$ is the current-current correlation function and

$$\hat{j}_x(\mathbf{r}, \tau) = -\mathrm{i}t_{sp} \sum_{\delta,\sigma} \left(P_\delta - \alpha\hat{u}_{\mathbf{r},\delta}\right) \left(s^\dagger_{\mathbf{r},\sigma} p_{\mathbf{r},\delta,\sigma} - h.c.\right) + \mathrm{i}t_{pp} \sum_{\delta,\delta',\sigma} Q_{\delta,\delta'} p^\dagger_{\mathbf{r},\delta,\sigma} p_{\mathbf{r},\delta',\sigma}, \tag{S14}$$

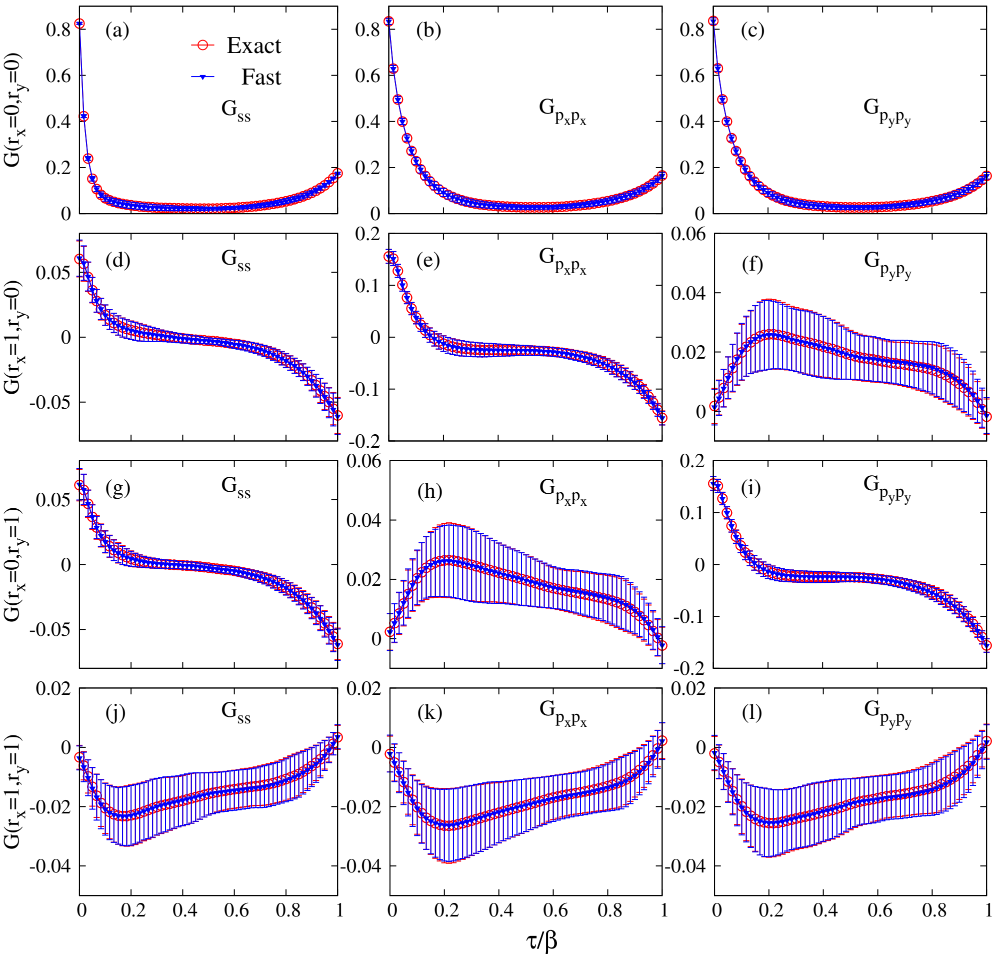


FIG. S1. (color online) Green's functions as a function of the imaginary time $\tau$ for different displacement $\mathbf{r} = r_x\mathbf{a} + r_y\mathbf{b}$. $\mathbf{a} = (a, 0)$ and $\mathbf{b} = (0, a)$ are the primitive vectors along the $x$- and $y$-directions, respectively, where $a$ is the Bi-Bi distance. The first, second, third columns show results for $G_{s,s}$, $G_{p_x,p_x}$,vand $G_{p_y,p_y}$, respectively. The red circles and blue triangles represent results obtained using the exact and fast update procedures, respectively. The error bars for the two approaches are comparable.

is the current operator, with phase factors $P_\delta$ (given in the main text) and $Q_{\pm x,\pm y} = -Q_{\pm y,\pm x} = -Q_{\pm x,\mp y} = Q_{\mp y,\pm x} = 1$.

A measure of the superconducting and charge ordering tendencies can be obtained from the orbitally-resolved charge $\chi^{\mathrm{C}}_{\gamma'\gamma}(\mathbf{q})$ and superconducting pair-field $\chi^{\mathrm{sc}}_{\gamma}$ susceptibilities, where $\gamma$ is an orbital index. The charge susceptibility is defined as

$$\chi^{\mathrm{C}}_{\gamma'\gamma}(\mathbf{q}) = \frac{1}{N}\int_0^\beta d\tau \langle \hat{n}_{\mathbf{q},\gamma'}(\tau)\hat{n}_{\mathbf{q},\gamma}(0)\rangle, \tag{S15}$$

where $\mathbf{q}$ is the momentum, $\tau$ is the imaginar ytime, $\hat{n}_{\mathbf{q},\gamma} = \sum_{i,\sigma} e^{\mathbf{i}\mathbf{q}\cdot\mathbf{r}_i}\hat{n}_{\mathbf{r}_i,\gamma,\sigma}$, and $\mathbf{r}_i$ is the lattice vector. Similarily, the pair-field susceptibility in the $s$-wave channel is given by

$$\chi^{\rm sc}_{\gamma} = \frac{1}{N}\int_0^\beta d\tau\langle\Delta_\gamma(\tau)\Delta^\dagger_\gamma(0)\rangle, \tag{S16}$$

where $\Delta_s = \sum_{\mathbf{r}} s_{\mathbf{r},\uparrow}s_{\mathbf{r},\downarrow}$ and $\Delta_{p_\delta} = \sum_{\mathbf{r}} p_{\mathbf{r},\delta,\uparrow}p_{\mathbf{r},\delta,\downarrow}$.

## S3. A molecular orbital viewpoint

To help understand DQMC results, we also carried out a simplified molecular orbital analysis of a $Bi_2O_4$ cluster, which provides a more transparent view of the physics. We refer the reader to Ref. [S5] for a similar discussion of the 3D case from an *ab initio* perspective. Note, however, that Ref. [S5] uses electron language whereas we use hole language.

The first step of our analysis is to expand the simple square unit cell to allow for two distinct Bi 6$s$ orbitals and four O 2$p$ orbitals, as indicated by the black dashed frame in Fig. S2(a). This expanded cell defines the cluster after we apply periodic boundary conditions. The two Bi 6$s$ orbitals are denoted as $s_1$ and $s_2$.

Next, we transform the four ligand oxygen orbitals into a molecular orbital basis using

$$\begin{aligned}
L_{\mathbf{r},s,\sigma} &= \frac{1}{2}(p_{\mathbf{r},x,\sigma} + p_{\mathbf{r},y,\sigma} - p_{\mathbf{r},-x,\sigma} - p_{\mathbf{r},-y,\sigma})\\
L_{\mathbf{r},d,\sigma} &= \frac{1}{2}(p_{\mathbf{r},x,\sigma} - p_{\mathbf{r},y,\sigma} - p_{\mathbf{r},-x,\sigma} + p_{\mathbf{r},-y,\sigma})\\
L_{\mathbf{r},x,\sigma} &= \frac{1}{\sqrt{2}}(p_{\mathbf{r},x,\sigma} + p_{\mathbf{r},-x,\sigma})\\
L_{\mathbf{r},y,\sigma} &= \frac{1}{\sqrt{2}}(p_{\mathbf{r},y,\sigma} + p_{\mathbf{r},-y,\sigma}).
\end{aligned}$$

(The $L_s$ and $L_d$ operators correspond to the $A_{1g}$ and $E_g$ orbitals in Ref. [S5].) Similarily, we can introduce new phonon operators

$$\begin{aligned}
\hat{x}_{\mathbf{r},L_s} &= \frac{1}{2}(\hat{u}_{\mathbf{r},x} + \hat{u}_{\mathbf{r},y} - \hat{u}_{\mathbf{r},-x} - \hat{u}_{\mathbf{r},-y})\\
\hat{x}_{\mathbf{r},L_d} &= \frac{1}{2}(\hat{u}_{\mathbf{r},x} + \hat{u}_{\mathbf{r},y} - \hat{u}_{\mathbf{r},-x} - \hat{u}_{\mathbf{r},-y})\\
\hat{x}_{\mathbf{r},L_x} &= \frac{1}{\sqrt{2}}(\hat{u}_{\mathbf{r},x} + \hat{u}_{\mathbf{r},-x})
\end{aligned}$$

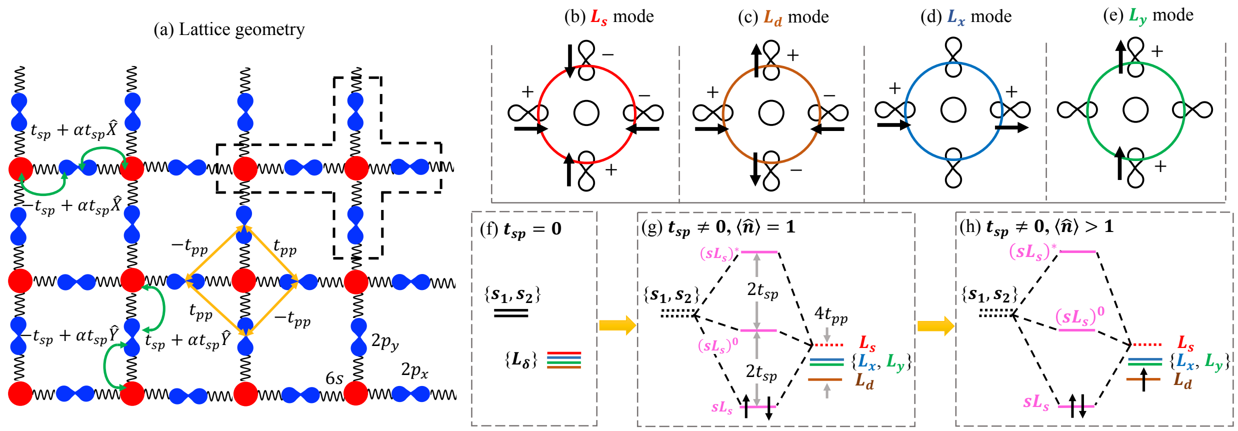


FIG. S2. (a) The lattice structure of the three-orbital model. (b) - (e) The phase factors of the $L_s$, $L_d$, $L_x$, and $L_y$ molecular orbitals, respectively, defined in our cluster analysis and the related oxygen vibrational modes. (f)-(h) Energy level diagrams of the four molecular orbitals and two Bi $6s$ orbitals. The case with (panel g) and without (panel f) hybridization between $6s$ and $2p_{x(y)}$ orbitals are shown. The black arrows indicate the hole occupations of the various levels at (g) half-filling $\langle \hat{n} \rangle = 1$ and (h) away from half-filling $\langle \hat{n} \rangle > 1$.

$$\hat{x}_{\mathbf{r},L_y} = \frac{1}{\sqrt{2}}(\hat{u}_{\mathbf{r},y} + \hat{u}_{\mathbf{r},-y}),$$

with analogous definitions for the momentum operators. Figs. S2(b)-S2(e) sketch the phases of the ligand $2p_\delta$ orbitals for each molecular orbital using $\pm$ signs, and the black arrows indicate the displacement patterns of the transformed phonon eigenmodes. The bond disproportionated structure that forms in the model corresponds to a coherent state of the optical $x_{\mathbf{r},L_s}$ phonon modes in this representation, while the $x_{\mathbf{r},L_x}$ and $x_{\mathbf{r},L_y}$ modes form the basis for the acoustic phonon modes.

After introducing the new basis and applying periodic boundary conditions, the Hamiltonian $H^M$ for the $Bi_2O_4$ cluster is $H^M = H_0^M + H_{\text{lat}}^M + H_{e-ph}^M$, where

$$\begin{aligned} H_0^M &= -2t_{sp}\sum_\sigma \left(s_{1,\sigma}^\dagger L_{s,\sigma} - s_{2,\sigma}^\dagger L_{s,\sigma} + h.c.\right) + (\epsilon_s - \mu)\sum_\sigma (\hat{n}_\sigma^{s_1} + \hat{n}_\sigma^{s_2}) \\ &\quad + (\epsilon_p - \mu)\sum_{\sigma,\alpha=x,y} \hat{n}_\sigma^{L_\alpha} + (\epsilon_p + 2t_{pp})\sum_\sigma \hat{n}_\sigma^{L_s} + (\epsilon_p - 2t_{pp})\sum_\sigma \hat{n}_\sigma^{L_d} \\ H_{\text{lat}}^M &= \sum_\gamma \left(\frac{1}{2M}\hat{p}_{L_\gamma}^2 + K\hat{x}_{L_\gamma}^2\right) \\ H_{e-ph}^M &= \alpha t_{sp}\sum_{\gamma,\sigma} \hat{x}_{L_\gamma}\left(s_{1,\sigma}^\dagger L_{\gamma,\sigma} + s_{2,\sigma}^\dagger L_{\gamma,\sigma} + h.c.\right). \end{aligned} \quad \text{(S17)}$$

Here, the sums on $\gamma$ are taken over $\gamma = s, d, x, y$ and $\hat{n}_\sigma^{L_\gamma} = L^\dagger_{\gamma,\sigma} L_{\gamma,\sigma}$.

We can glean several insights into the problem from this cluster model. In the atomic limit ($t_{sp} = t_{pp} = 0$) and in the negative charge transfer regime ($\epsilon_p < \epsilon_s$ in hole language), the four molecular orbitals are degenerate, as shown in Fig. S2(f). This degeneracy is lifted by the orbital overlaps: a nonzero $t_{pp}$ raises (lowers) the onsite energy of the $L_s$ ($L_d$) molecular orbital, while a nonzero $t_{sp}$ hybridizes the Bi $s$ and molecular $L_s$ orbitals to form new bonding ($sL_s$), nonbonding $(sL_S)^0$, and antibonding $(sL_s)^*$ states. Here, the bonding state's energy is lowered by $2t_{sp}$ relative to the atomic values such that the two holes fill this state at half-filling, as shown in Fig. S2(g). This ground state charge distribution is analogous to the one inferred for 3D bismuthates in *ab initio* calculations [S5] and ARPES measurements [S6].

The impact of the $e$-ph coupling is also evident from this form of the Hamiltonian; holes hop between the $L_\gamma$ molecular orbital and the Bi sites while exciting phonon eigenmodes with the same symmetry. At half-filling, the holes in the ($sL_s$) bonding state will, therefore, excite the breathing phonon mode of the surrounding oxygen atoms. In an extensive system, this coupling can lead to a static breathing distortion of the lattice after a spontaneous symmetry breaking selects one of the Bi sublattices as the center of the compressed plaquettes. Upon doping, the additional holes will occupy the $L_d$ and $L_{x,y}$ orbitals, where they will couple to the orthogonal phonon modes. Since the superposition of the individual modes determines the total displacement of the oxygen atoms, the breathing distortion will relax as the other modes are excited, even though the ($sL_s$) holes remain coupled to the $x_{L_s}$ phonons.

To confirm this physical picture, we diagonalized the Hamiltonian $H^M$ on a $Bi_2O_4$ cluster and evaluated several observables in the grand canonical ensemble, with $\beta = 14.56/t_{sp}$, $\Omega = t_{sp}$, and $\mu$ was adjusted to set the particle number. When diagonalizing this model, we included up to $N_{ph} = 5$ quanta for *each* phonon mode, which was sufficient to obtain converged results for our choice of parameters.

Figure S3 summarizes the results of our exact diagonlization (ED) calculations. Figure S3(a) and S3(b) plot the evolution of the hole density $\langle \hat{n}^{L_\gamma} \rangle$ on each molecular orbital, and the displacement fluctuations of each eigenmode $\delta(x_\delta) = \langle \hat{x}^2_{L_\delta} \rangle - \langle \hat{x}_{L_\delta} \rangle^2$, respectively, as a function of the total filling. As expected, the holes primarily occupy the $L_s$ orbital at half-filling. (The missing hole weight is split between the two Bi sites and is not shown.) At the same time, the displacement of the $x_{L_s}$ mode fluctuates significantly, while the

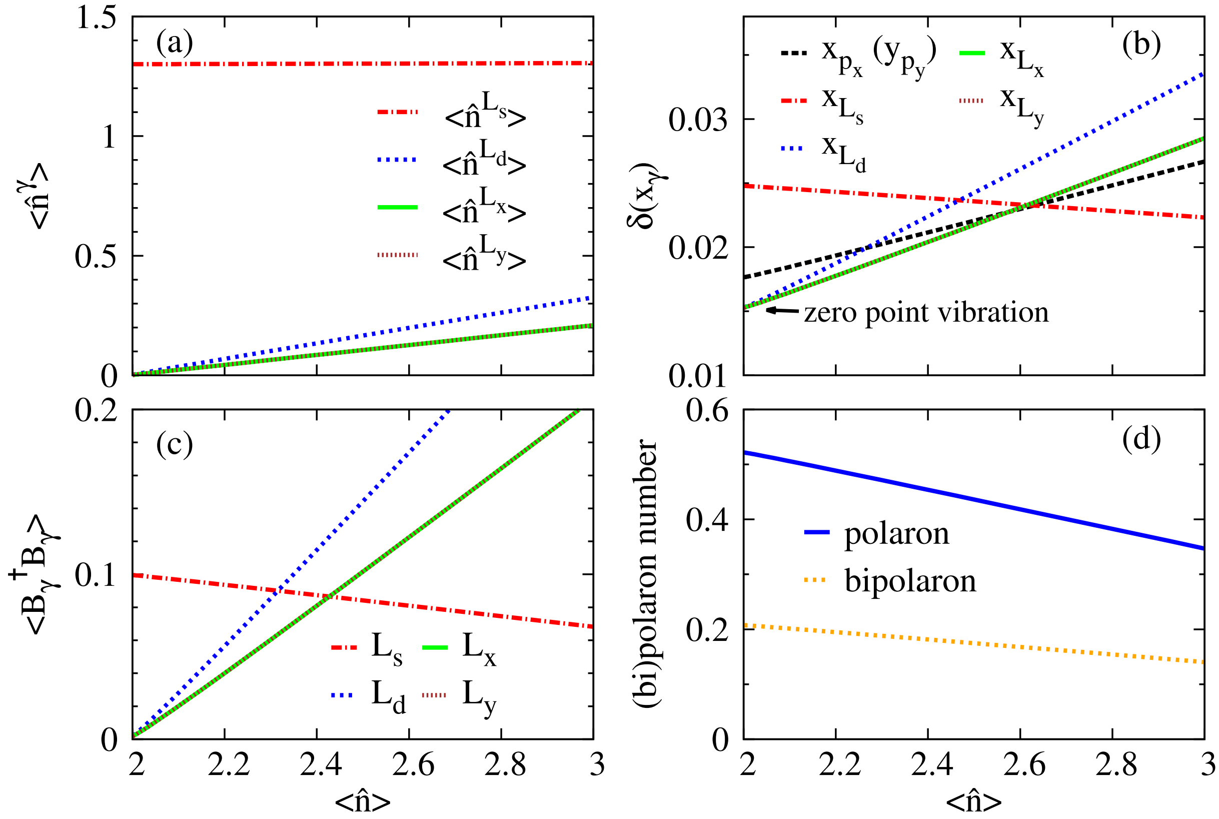


FIG. S3. Exact diagonalization results for the $Bi_2O_4$ cluster as a function of the total filling and temperature of $\beta = 14.56/t_{sp}$. (a) The hole density on each molecular orbital as a function of doping. The missing hole weight is located equally on the Bi orbitals and is not shown. (b) The average fluctuation of the atomic displacement associated with each of the four eigenmodes shown in Fig. S2. (c) The average number of phonon quanta in the cluster. (d) The expectation value of the polaron and bipolaron operators defined in the main text.

remaining eigenmodes have fluctuations consistent with zero point motion. This behavior is also reflected in the expectation value of the phonon numbers [Fig. S3(c)], where the $x_{L_s}$ modes are excited while the remaining phonon modes are in their ground state. Note that we do not observe a nonzero $\langle \hat{x}_{L_s} \rangle \neq 0$ due to the absence of any symmetry breaking in the cluster; however, our DQMC simulations performed on larger lattices do find such a state.

When additional holes are introduced they enter the $L_d$, $L_x$ and $L_y$ molecular orbitals, as expected based on the level diagram shown in Fig. 1(h). In this case, the $L_d$ orbital has a larger hole occupation due to the finite value of $t_{pp}$. At the same time, $\delta(x_{L_d})$, $\delta(x_{L_x})$, and $\delta(x_{L_d})$ also increase linearly and the number phonon quanta for these modes grows. Both the displacement fluctuations and the number of excited phonon quanta are comparable for the four phonon modes once the hole doping reaches $\langle \hat{n} \rangle = 2.4 - 2.6$. Finally, the introduction

of additional holes slightly suppresses the magnitude of $\delta(x_{L_s})$ and the total number of $x_{L_s}$ modes.

Our ED calculations suggest that hole doping induces relaxation of the breathing distortion of the lattice, which is dominant at half-filling. However, it does so by exciting the orthogonal phonon modes rather than by suppressing the number of $x_{L_s}$ quanta in the system. In this context, it is interesting then to determine if the $L_s$ holes and $x_{L_s}$ modes can be viewed of as a composite object (*i.e.*, a polaron). We checked this idea in our ED calculations by computing the expectation value of the polaron $P$ and bipolaron $BP$ number operators, defined as

$$\langle P\rangle = \langle(\hat{n}^{s_1} + \hat{n}^{L_s})\hat{x}_{L_s} - (\hat{n}^{s_2} + \hat{n}^{L_s})\hat{x}_{L_s}\rangle \tag{S18}$$

and

$$\langle BP\rangle = \langle(\hat{n}^{s_1}_{\uparrow} + \hat{n}^{L_s}_{\uparrow})(\hat{n}^{s_1}_{\downarrow} + \hat{n}^{L_s}_{\downarrow})\hat{x}_{L_s} - (\hat{n}^{s_2}_{\uparrow} + \hat{n}^{L_s}_{\uparrow})(\hat{n}^{s_2}_{\downarrow} + \hat{n}^{L_s}_{\downarrow})\hat{x}_{L_s}\rangle. \tag{S19}$$

These operators measure the combined presence of holes in the $(sL_s)$ bonding orbital together with a compression of the ligand oxygens. (The same quantities are also measured in our DQMC calculations [see Fig. 3(b)] in the main text.) Here, the minus sign in front of the second terms accounts for the fact that a compression of the O atoms around the second Bi site corresponds to a negative displacement of the $x_{L_s}$ mode as we have defined it. Fig. S3(d) plots the doping evolution of the $\langle P\rangle$ and $\langle BP\rangle$. We find that the ground state has a significant amount of polaron and bipolaron character, which persists to higher doping levels. Our ED results strongly suggest that the system hosts polaronic carriers, where holes occupying the $L_s$ molecular orbitals are bound to local $x_{L_s}$ modes.

The molecular orbitals discussed here will of course form bands in the extended system. Nevertheless, much of our analysis still applies in this case. To illustrate this, Fig. S4 plots the non-interacting band structure of our model in the insulating phase, where the bond disproportionated structure has been introduced by modifying the hopping integrals as $t^{ij}_{sp} = t_{sp}\,[1 + (-1)^{i+j} \times 0.3]$. Fig. S4(a) and Fig. S4(b) provide fat band plots of the $L_s$ and $L_d$ molecular orbital weight, respectively, while Fig. S4(c) plots the total and orbitally-resolved density of states (DOS). As can be seen in Fig. S4(a), the occupied band below the Fermi level ($E = 0$) at half-filling is the bonding $(sL_s)$ band, which couples to the breathing motion of the lattice. The first band above the Fermi level is mostly of $L_d$ and $L_{x,y}$ orbital character, such that doped holes will predominantly couple to the corresponding phonon

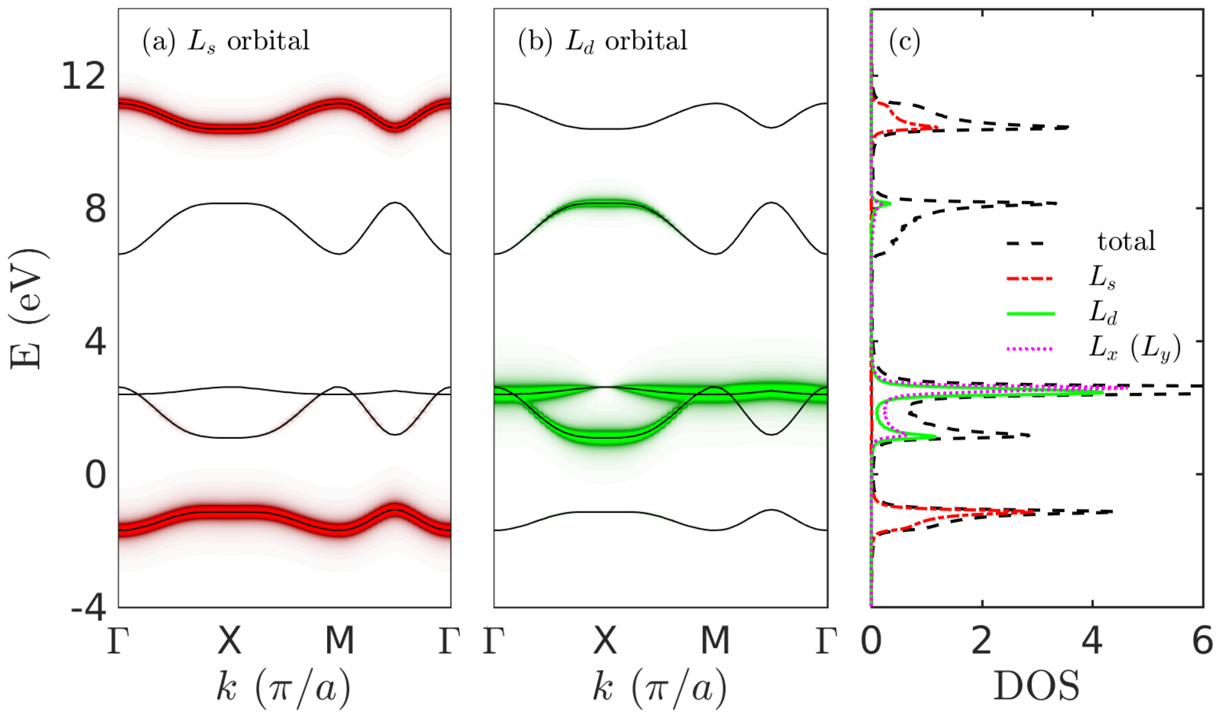


FIG. S4. (color online) The non-interacting band structure of the two-dimensional *sp*-model in the insulating (bond disproportionated) state and in hole language. Panels (a) and (b) are fat band plots showing the $L_s$ and $L_d$ weight of each of the bands, respectively. Panel (c) is the total DOS and its orbital components. The completely occupied band below the Fermi level is the Bi $6s/L_s$ bonding band orbitals. The first band above the Fermi level is composed of $L_{x,y}$ and $L_d$ orbitals.

modes.

Reviewing our DQMC results, we suggest that the suppression of long-range polaron and bipolaron correlations with hole doping should be induced by introducing other phonon modes rather than directly suppressing the breathing phonon mode. We also note that the orbital character and electronic structure of $BaBiO_3$ computed with *ab initio* methods share many similarities to the plot shown in Fig. S4. This fact suggests that our analysis can be extended to the bulk 3D material.

[S1] S. R. White, D. J. Scalapino, R. L. Sugar, E. Y. Loh, J. E. Gubernatis, and R. T. Scalettar, Phys. Rev. B **40**, 506 (1989).

[S2] S. Johnston, E. A. Nowadnick, Y. F. Kung, B. Moritz, R. T. Scalettar, and T. P. Devereaux, Phys. Rev. B **87**, 235133 (2013).

[S3] R. Blankenbecler, D. J. Scalapino, and R. L. Sugar, Phys. Rev. D **24**, 2278 (1981).

[S4] N. Trivedi, R. T. Scalettar, and M. Randeria, Phys. Rev. B **54**, R3756 (1996).

[S5] K. Foyevtsova, A. Khazraie, I. Elfimov, and G. A. Sawatzky, Phys. Rev. B **91**, 121114 (2015).

[S6] N. C. Plumb, D. J. Gawryluk, Y. Wang, Z. Ristić, J. Park, B. Q. Lv, Z. Wang, C. E. Matt, N. Xu, T. Shang, K. Conder, J. Mesot, S. Johnston, M. Shi, and M. Radović, Phys. Rev. Lett. **117**, 037002 (2016).
